# Supplementary material for: Gossip Dual Averaging for Decentralized Optimization of Pairwise Functions
Source: arXiv:1606.02421 source file (2016-06-08)
Supplement: Supplementary file 1 [file additional_results.tex]

\section{Additional Results}
\label{sec:additional-results}

\subsection{Convergence of Gradient Variables}
\label{sec:conv-grad-vari}

Theorem~\ref{thm:dist_dual_averaging_general_rate} provides a convergence rate in two distinct part. First, an optimization term, which is exactly the same than in the centralized setting. Then, a network-dependent term which depends on the global variation of the dual variables; the following lemma provides an explicit dependence between this term and the topology of the network.
\begin{lemma}
  Let $W \in \bbR^{n \times n}$ be a doubly stochastic matrix satisfying~\eqref{eq:w_condition}. Let $(Z(t))_{t > 0}$ and $(G(t))_{t > 0}$ satisfying the update rule~\eqref{eq:dist_dual_matrix_update}. Then, for $t > 0$, one has:
  \[
    \left\| Z(t) - \1_n \overline{z}^n(t)^{\top} \right\| \leq \sum_{s = 1}^t \lambda_2(W)^{t - s} \|G(s - 1)\|,
  \]
  where $\lambda_2(W)$ is the second largest eigenvalue of $W$. Moreover, if $\mathcal{G}$ is connected and non bipartite and if there exists $L > 0$ such that for any $s > 0$, $\|G(s)\|_{\infty} \leq L$, then one has:
  \[
    \left\| Z(t) - \1_n \overline{z}^n(t)^{\top} \right\|_{\infty} \leq \frac{L}{1 - \lambda_2(W)}.
  \]
\end{lemma}

\subsection{Stochastic Gradient}
\label{sec:stochastic-gradient}

Again, the decentralized setting can be adapted to a stochastic setting, where each node compute an unbiased estimator of the gradient.

\begin{theorem}
  \label{thm:dist_dual_averaging_stoch_rate}
  Let $(\gamma(t))_{t \geq 0} \in (\bbR_+^*)^{\bbN}$ be a non increasing sequence. For $i \in [n]$, let $(g_i(t))_{t \geq 0} \in (\bbR^d)^{\bbN}$, $(z_i(t))_{t \geq 0} \in (\bbR^d)^{\bbN}$ and $(x_i(t))_{t > 0} \in (\bbR^d)^{\bbN}$ be generated according to Algorithm~\ref{alg:dist_dual_averaging_sto}. For $x^* \in \argmin_{x \in \mathcal{Q}} \overline{f}^n(x)$, $i \in [n]$ and $T > 0$, one has:
  \[
    \bbE_T[\overline{f}^n(\overline{x}^T_i) - \overline{f}^n(x^*)] \leq C_1(T) + C_2(T) 
  \]
  where
  \[
    \left\{
      \begin{aligned}
        C_1(T) &= \frac{1}{2 T \gamma(T)} \| x^* \|^2 + \frac{L_f^2}{2T} \sum_{t = 1}^T \gamma(t - 1) z_j(t) \| \Big] \\
        C_2(T) &=  \frac{1}{n} \sum_{j = 1}^n \bbE_t\Big[ \|z_i(t) - z_j(t) \| + \| \overline{z}^n(t) - z_j(t) \| \Big]
    \end{aligned}
    \right.
  \]
\end{theorem}

\subsection{Biased Stochastic Gradient}
\label{sec:bias-stoch-grad}

We now focus on the case where the descent direction is stochastic but also a \emph{biased} estimate of the gradient. That is, instead of updating a dual variable $z_i(t)$ with $g_i(t)$ such that $\bbE[g_i(t) | x_i(t)] \in \partial f_i(x_i(t))$, we perform some update $d_i(t)$, and we denote $\epsilon_i(t)$ the quantity such that $\bbE[d_i(t) - \epsilon_i(t) | x_i(t)] = \bbE[g_i(t) | x_i(t)] \in \partial f_i(x_i(t))$. The following theorem allows to upperbound the error induced by the bias.

\begin{theorem}
  \label{thm:dist_dual_averaging_stoch_biased_rate}
  Let $(\gamma(t))_{t \geq 0} \in (\bbR_+^*)^{\bbN}$ be a non increasing sequence. For $i \in [n]$, let $(d_i(t))_{t \geq 0} \in (\bbR^d)^{\bbN}$, $(g_i(t))_{t \geq 0} \in (\bbR^d)^{\bbN}$, $(\epsilon_i(t))_{t \geq 0} \in (\bbR^d)^{\bbN}$, $(z_i(t))_{t \geq 0} \in (\bbR^d)^{\bbN}$ and $(x_i(t))_{t > 0} \in (\bbR^d)^{\bbN}$ be generated as stated previously. For $x^* \in \argmin_{x \in \mathcal{Q}} \overline{f}^n(x)$, $i \in [n]$ and $T > 0$, one has:
  \[
    \bbE_T[\overline{f}^n(\overline{x}^T_i) - \overline{f}^n(x^*)] \leq C_1(T) + C_2(T) + C_3(T),
  \]
  where
  \[
    \left\{
      \begin{aligned}
        C_1(T) &= \frac{1}{2 T \gamma(T)} \| x^* \|^2 + \frac{L_f^2}{2T} \sum_{t = 1}^T \gamma(t - 1) \\
        C_2(T) &= \frac{L_f}{nT} \sum_{t = 1}^T \gamma(t - 1) \sum_{j = 1}^n \bbE\Big[ \|z_i(t) - z_j(t) \| + \| \overline{z}^n(t) - z_j(t) \| \Big] \\
        C_3(T) &= \frac{1}{T} \sum_{t = 1}^{T} \bbE_t[\|y(t) - x^*\| \| \overline{\epsilon}^n(t) \|].
      \end{aligned}
    \right.
  \]  
\end{theorem}

%%% Local Variables:
%%% mode: latex
%%% TeX-master: "../main"
%%% End:
